# Supplementary material for: DeClotH: Decomposable 3D Cloth and Human Body Reconstruction from a Single Image
Source: arXiv:2503.19373 source file (2025-03-25)
Supplement: Supplementary file 1 [file eval_clothing.tex]

\begin{table}[t]

\footnotesize
\begin{center}
\scalebox{0.71}{
    \begin{tabular}{>{\raggedright\arraybackslash}m{2.1cm}|>{\centering\arraybackslash}m{1.0cm}>{\centering\arraybackslash}m{1.0cm}|>{\centering\arraybackslash}m{1.05cm}>{\centering\arraybackslash}m{1.05cm}|>{\centering\arraybackslash}m{1.0cm}>{\centering\arraybackslash}m{1.0cm}|>{\centering\arraybackslash}m{1.05cm}>{\centering\arraybackslash}m{1.05cm}}
    \specialrule{.1em}{.05em}{0.0em}
    &&&&&&\\[-3.8mm]
        &  \multicolumn{2}{c|}{\makecell[c]{4D-DRESS\\(cloth)}} & \multicolumn{2}{c|}{\makecell[c]{4D-DRESS\\(cloth+human)}} & \multicolumn{2}{c|}{\makecell[c]{THuman2.0\\(cloth)}} & \multicolumn{2}{c}{\makecell[c]{THuman2.0\\(cloth+human)}} \\
        Methods & CD$^{\downarrow}$ & NC$^{\downarrow}$ & CD$^{\downarrow}$ & NC$^{\downarrow}$ & CD$^{\downarrow}$ & NC$^{\downarrow}$ & CD$^{\downarrow}$ & NC$^{\downarrow}$ \\
        \hline
        BCNet$^{\dagger}$~\cite{jiang2020bcnet} & 3.987 & 0.046 & 3.925 & 0.088 & 1.906 & 0.046 & 2.090 & 0.098 \\
        SMPLicit~\cite{corona2021smplicit} & 4.080 & 0.038 & 3.605 & 0.091 & 1.601 & 0.044 & 1.744 & 0.094  \\
        ClothWild~\cite{moon20223d} & 3.940 & 0.037 & 3.493 & 0.087 & 1.578 & 0.042 & 1.600 & 0.086 \\
        \textbf{\ourmethod~$^{\dagger}$(Ours)}  & \textbf{0.000} & \textbf{0.000} & \textbf{0.000} & \textbf{0.000} & \textbf{0.000} & \textbf{0.000} & \textbf{0.000} & \textbf{0.000} \\
        \textbf{\ourmethod~(Ours)} & \textbf{0.000} & \textbf{0.000} & \textbf{0.000} & \textbf{0.000} & \textbf{0.000} & \textbf{0.000} & \textbf{0.000} & \textbf{0.000} \\
        \specialrule{.1em}{-0.05em}{-0.05em}
    \end{tabular}   
}
\end{center}
    \vspace*{-1.4em}
    \caption{
        \textbf{Quantitative comparison with existing 3D clothing reconstruction methods.}
        $\dagger$ denotes that shoes are excluded from the evaluation.
    }
    \vspace*{-1.0em}
    \label{tab:eval_recon}
\end{table}
